# Supplementary material for: BCFA: Bespoke Control Flow Analysis for CFA at Scale
Source: arXiv:2005.01000 source file (2020-05-03)
Supplement: Supplementary file 1 [file appendix.tex]

\section{Appendix}
\label{sec:appendix}
\input{tex-figures/paths-table2.tex}
\input{prediction-precision}
\input{tex-figures/loop-precision}
